# Supplementary material for: Second order semi-parametric inference for multivariate log Gaussian Cox processes
Source: arXiv:2012.02155 source file (2022-01-03)
Supplement: Supplementary file 1 [file appendix.tex]

\section{Theoretical results}
\begin{lemma}\label{lem:unb}
The estimating function $\nabla_{\balpha} l_-(\btheta^*)=\best(\btheta^*)$ with respect to $\balpha$ is unbiased.
\end{lemma}

\begin{proof}
\begin{align*}
\textup{E}[\best(\btheta^*)] &=  \textup{E} \left[ \sum_{i \leq j} \sum_{\substack{\bu \in X_i \cap W\\ \bv \in X_j \cap W}}^{\neq} \left( \frac{\sum_{k \leq l} \nabla_{\balpha} \rho_{kl}(\bu,\bv;\btheta_{kl}^*)}{\sum_{k \leq l}  \rho_{kl}(\bu,\bv;\btheta_{kl}^*)} - \frac{\nabla_{\balpha} \rho_{ij}(\bu,\bv;\btheta_{ij}^*)}{\rho_{ij}(\bu,\bv;\btheta_{ij}^*)} \right) \right] \\
& = \sum_{i \leq j} \int_{W^2} \left( \frac{\sum_{k \leq l} \nabla_{\balpha} \rho_{kl}(\bu,\bv;\btheta_{kl}^*)}{\sum_{k \leq l}  \rho_{kl}(\bu,\bv;\btheta_{kl}^*)} - \frac{\nabla_{\balpha} \rho_{ij}(\bu,\bv;\btheta_{ij}^*)}{\rho_{ij}(\bu,\bv;\btheta_{ij}^*)}  \right)\rho_{ij}(\bu,\bv;\btheta_{ij}^*) \textup{d}\bu \textup{d}\bv \\
&=   \int_{W^2}  \sum_{k \leq l} \nabla_{\balpha} \rho_{kl}(\bu,\bv;\btheta_{kl}^*) - \sum_{i \leq j} \nabla_{\balpha} \rho_{ij}(\bu,\bv;\btheta_{ij}^*) \textup{d}\bu \textup{d}\bv = \boldsymbol{0}.
\end{align*}
\end{proof}

\begin{lemma}\label{prop:sens}
The expected hessian matrix of $l_-(\btheta^*)$ with respect to $\balpha$ is given by:
\begin{align*}
\textup{H}(\btheta^*)=\int_{W^2}\textup{Cov}(X(\bu,\bv,\btheta^*))  \sum_{i \leq j} \rho_{ij}(\bu,\bv;\btheta^*) \textup{d} \bu \textup{d} \bv,
\end{align*}
where for each $\bu$, $\bv$, $X(\bu,\bv,\btheta^*)$ denote a random vector which takes values $\nabla_{\balpha} \textup{log}(\rho_{ij}(\bu,\bv; \btheta^*))$ with probabilities $\textup{p}_{ij}(\bu,\bv; \btheta^*)$, $i=1, \cdots,qp$.
\end{lemma}

\begin{proof}
We suppress the arguments $\bu$, $\bv$ and $\btheta^*$ in order to save space. The hessian matrix for $l_-(\btheta^*)$ is:
\begin{align*}
&\frac{\partial}{\partial \balpha^T} e(\btheta)= \nabla^2_{\balpha} l_-(\btheta)= \\
& \sum_{i \leq j} \sum_{\substack{\bu \in X_i \cap W \\ \bv \in X_j \cap W}} \frac{( \sum_{k \leq l} \nabla^2_{\balpha}  \rho_{kl} ) (\sum_{k \leq l} \rho_{kl}) - (\sum_{k \leq l} \nabla_{\balpha}  \rho_{kl})( \sum_{k \leq l} \nabla^T_{\balpha}  \rho_{kl})  }{(\sum_{k  \leq l} \rho_{kl})^2} \quad -\\
& \sum_{i \leq j} \sum_{\substack{\bu \in X_i \cap W \\ \bv \in X_j \cap W}}  \frac{ (\nabla^2_{\balpha} \rho_{ij}) \rho_{ij} - (\nabla_{\balpha} \rho_{ij}) (\nabla^T_{\balpha} \rho_{ij})}{\rho_{ij}^2} 
\end{align*}
The expected hessian is the given by:
\begin{align*}
& \textup{H}(\btheta^*) \\
= & \sum_{i  \leq j} \int_{W^2} 1_R \frac{( \sum_{k \leq l} \nabla^2_{\balpha}  \rho_{kl} ) (\sum_{k  \leq l} \rho_{kl}) - (\sum_{k \leq l} \nabla_{\balpha}  \rho_{kl})( \sum_{k \leq l} \nabla^T_{\balpha}  \rho_{kl})  }{(\sum_{k \leq l} \rho_{kl})^2} \rho_{ij} du dv \quad -\\  & \sum_{i \leq j} \int_{W^2} 1_R \frac{ (\nabla^2_{\balpha} \rho_{ij}) \rho_{ij} - (\nabla_{\balpha} \rho_{ij}) (\nabla^T_{\balpha} \rho_{ij})}{\rho_{ij}^2} \rho_{ij} du dv \\
= & \int_{W^2} 1_R \sum_{i \leq j} \frac{ (\nabla_{\balpha} \rho_{ij}) (\nabla^T_{\balpha} \rho_{ij})}{\rho_{ij}} - \frac{(\sum_{k \leq l} \nabla_{\balpha}  \rho_{kl})( \sum_{k \leq l} \nabla^T_{\balpha}  \rho_{kl})  }{\left( \sum_{k \leq l} \rho_{kl} \right)} du dv \\
= & \int_{W^2} 1_R \left( \sum_{k \leq l} \rho_{kl} \right) \left( \sum_{i , j} \nabla_{\balpha} \textup{log}(\rho_{ij}) \nabla^T_{\balpha} \textup{log} (\rho_{ij}) \textup{p}_{ij} - (\sum_{k \leq l} \nabla_{\balpha}  \textup{log} ( \rho_{kl})\textup{p}_{kl}) ( \sum_{k \leq l} \nabla_{\balpha} \textup{log} (\rho_{kl})\textup{p}_{kl} )^T \right) du dv \\
= & \int_{W^2} 1_R \left( \sum_{i \leq j} \rho_{ij} \right) \textup{Cov}(X(u,v,\btheta^*)) du dv.
\end{align*}
\end{proof}

\section{Quadratic approximation of likelihood} \label{app:pnm}
We can rewrite \eqref{eq:loglik} as a least squares problem. When taking a closer look at \eqref{eq:taylor}, we see that:
\begin{align} 
\hat{\bpsi} \approx &\textup{arg min}_{\bpsi} \bigg( f(\bpsi,\bpi^{(n)}) \bigg) \label{eq:taylorapp} \\
 \equiv & \textup{arg min}_{\bpsi} \bigg( (\bpsi - \bpsi^{(n)})^T \best(\bpsi^{(n)},\bpi^{(n)})+ \frac{1}{2}(\bpsi - \bpsi^{(n)})^T \textup{H} (\bpsi^{(n)},\bpi^{(n)})(\bpsi - \bpsi^{(n)}) \bigg) \nonumber\\
 \equiv & \textup{arg min}_{\bpsi} \bigg( -(\bpsi - \bpsi^{(n)})^T  \textup{H} (\bpsi^{(n)},\bpi^{(n)})K + \frac{1}{2}(\bpsi - \bpsi^{(n)})^T \textup{H} (\bpsi^{(n)},\bpi^{(n)})(\bpsi - \bpsi^{(n)}) \bigg) \nonumber\\
 \equiv & \textup{arg min}_{\bpsi} \bigg( \frac{1}{2}(K-(\bpsi - \bpsi^{(n)}))^T \textup{H} (\bpsi^{(n)},\bpi^{(n)})(K-(\bpsi - \bpsi^{(n)})) \bigg) \nonumber,
\end{align}
where $K=-\textup{H}^{-1}(\bpsi^{(n)},\bpi^{(n)})\best(\bpsi^{(n)},\bpi^{(n)})$. Hence, we see \eqref{eq:taylorapp} is a least squares problem:
\begin{align} 
\hat{\bpsi} \approx & \textup{arg min}_{\bpsi} \bigg(\frac{1}{2} ||\textup{H} (\bpsi^{(n)},\bpi^{(n)})^{1/2}(K-(\bpsi- \bpsi^{(n)}))||^2 \bigg) \nonumber\\
\equiv & \textup{arg min}_{\bpsi} \bigg( \frac{1}{2} ||Y -X\bpsi ||^2 \bigg) ,
\end{align}
where
\begin{align*}
Y&=\textup{H}(\bpsi^{(n)},\bpi^{(n)})^{1/2}\left( -\textup{H}(\bpsi^{(n)},\bpi^{(n)})^{-1}\best(\bpsi^{(n)},\bpi^{(n)})+\bpsi^{(n)} \right) \quad \textup{and} \\
X&=\textup{H}(\bpsi^{(n)},\bpi^{(n)})^{1/2}.
\end{align*}
