# Supplementary material for: Second order semi-parametric inference for multivariate log Gaussian Cox processes
Source: arXiv:2012.02155 source file (2022-01-03)
Supplement: Supplementary file 2 [file litteratur.tex]

\chapter{Litteratur} \nonumber

Møller, J. \& Waagepetersen, R. P. (2004). $Statistical$ $Inference$ $and$ $Simulation$ $for$ $Spatial$ $Point$ $Processes$. Chapman \& Hall/CRC. 1. udgave.
\\

\noindent van Lieshout, M. (2010). $Spatial$ $Point$ $Process$ $Theory$. Handbook of Spatial Statistics. CRC Press, 263-282.
