# Supplementary material for: Second order semi-parametric inference for multivariate log Gaussian Cox processes
Source: arXiv:2012.02155 source file (2022-01-03)
Supplement: Supplementary file 3 [file hyphenations.tex]

% see, e.g., http://en.wikibooks.org/wiki/LaTeX/Formatting#Hyphenation
% for more information on word hyphenation
\hyphenation{ex-am-ple hy-phen-a-tion short}
\hyphenation{long la-tex}
\hyphenation{gen-e-ra-li-ty}
\hyphenation{li-ke-li-ho-od-funk-ti-on}
\hyphenation{log-li-ke-li-ho-od-funk-ti-on}
\hyphenation{es-ti-ma-ti-ons-funk-ti-on-er}
