# Supplementary material for: Second order semi-parametric inference for multivariate log Gaussian Cox processes
Source: arXiv:2012.02155 source file (2022-01-03)
Supplement: Supplementary file 5 [file macros.tex]

%  A simple AAU report template.
%  2014-09-13 v. 1.1.0
%  Copyright 2010-2014 by Jesper KjÃ¦r Nielsen <jkn@es.aau.dk>
%
%  This is free software: you can redistribute it and/or modify
%  it under the terms of the GNU General Public License as published by
%  the Free Software Foundation, either version 3 of the License, or
%  (at your option) any later version.
%
%  This is distributed in the hope that it will be useful,
%  but WITHOUT ANY WARRANTY; without even the implied warranty of
%  MERCHANTABILITY or FITNESS FOR A PARTICULAR PURPOSE.  See the
%  GNU General Public License for more details.
%
%  You can find the GNU General Public License at <http://www.gnu.org/licenses/>.
%
%
%
% see, e.g., http://en.wikibooks.org/wiki/LaTeX/Customizing_LaTeX#New_commands
% for more information on how to create macros

%%%%%%%%%%%%%%%%%%%%%%%%%%%%%%%%%%%%%%%%%%%%%%%%
% Macros for the titlepage
%%%%%%%%%%%%%%%%%%%%%%%%%%%%%%%%%%%%%%%%%%%%%%%%
%Creates the aau titlepage
\newcommand{\aautitlepage}[3]{%
  {
    %set up various length
    \ifx\titlepageleftcolumnwidth\undefined
      \newlength{\titlepageleftcolumnwidth}
      \newlength{\titlepagerightcolumnwidth}
    \fi
    \setlength{\titlepageleftcolumnwidth}{0.5\textwidth-\tabcolsep}
    \setlength{\titlepagerightcolumnwidth}{\textwidth-3\tabcolsep-\titlepageleftcolumnwidth}
    %create title page
    \thispagestyle{empty}
    \noindent%
    \begin{tabular}{@{}ll@{}}
      \parbox{\titlepageleftcolumnwidth}{
        \iflanguage{danish}{%
          \includegraphics[width=\titlepageleftcolumnwidth]{figures/aau_logo_da}
        }{%
          \includegraphics[width=\titlepageleftcolumnwidth]{figures/aau_logo_en}
        }
      } &
      \parbox{\titlepagerightcolumnwidth}{\raggedleft\sf\small
        #2
      }\bigskip\\
       #1 &
      \parbox[t]{\titlepagerightcolumnwidth}{%
      \textbf{Abstract:}\bigskip\par
        \fbox{\parbox{\titlepagerightcolumnwidth-2\fboxsep-2\fboxrule}{%
          #3
        }}
      }\\
    \end{tabular}
    \vfill
    \iflanguage{danish}{%
      \noindent{\footnotesize\emph{Rapportens indhold er frit tilgængeligt, men offentliggørelse (med kildeangivelse) må kun ske efter aftale med forfatterne.}}
    }{%
      \noindent{\footnotesize\emph{The content of this report is freely available, but publication (with reference) may only be pursued due to agreement with the author.}}
    }
    \clearpage
  }
}

%Create english project info
\newcommand{\englishprojectinfo}[8]{%
  \parbox[t]{\titlepageleftcolumnwidth}{
    \textbf{Title:}\\ #1\bigskip\par
    \textbf{Theme:}\\ #2\bigskip\par
    \textbf{Project Period:}\\ #3\bigskip\par
    \textbf{Project Group:}\\ #4\bigskip\par
    \textbf{Participants:}\\ #5\bigskip\par
    \textbf{Supervisor:}\\ #6\bigskip\par
    \textbf{Copies:} #7\bigskip\par
    \textbf{Page Numbers: }\pageref{LastPage}  \bigskip\par
    \textbf{Date of Completion:}\\ #8
  }
}

%Create danish project info
\newcommand{\danishprojectinfo}[8]{%
  \parbox[t]{\titlepageleftcolumnwidth}{
    \textbf{Titel:}\\ #1\bigskip\par
    \textbf{Tema:}\\ #2\bigskip\par
    \textbf{Projektperiode:}\\ #3\bigskip\par
    \textbf{Projektgruppe:}\\ #4\bigskip\par
    \textbf{Deltager:}\\ #5\bigskip\par
    \textbf{Vejleder:}\\ #6\bigskip\par
    \textbf{Oplagstal:} #7\bigskip\par
    \textbf{Sidetal:} \pageref{LastPage}  \bigskip\par
    \textbf{Afleveringsdato:}\\ #8
  }
}

%%%%%%%%%%%%%%%%%%%%%%%%%%%%%%%%%%%%%%%%%%%%%%%%
% An example environment
%%%%%%%%%%%%%%%%%%%%%%%%%%%%%%%%%%%%%%%%%%%%%%%%
\theoremheaderfont{\normalfont\bfseries}
\theorembodyfont{\normalfont}
\theoremstyle{break}
\def\theoremframecommand{{\color{aaublue!50}\vrule width 5pt \hspace{5pt}}}


\newshadedtheorem{sat}{Theorem}[section]
\newenvironment{satning}{%
		\begin{sat}
}{%
		\end{sat}
}


\newshadedtheorem{prop}[sat]{Proposition}
\newenvironment{proposition}{%
		\begin{prop}
}{%
		\end{prop}
}

\newshadedtheorem{lem}[sat]{Lemma}
\newenvironment{lemma}{%
		\begin{lem}
}{%
		\end{lem}
}

\newshadedtheorem{mydef}[sat]{Definition}
\newenvironment{definition}[1]{%
		\begin{mydef}[#1]
}{%
		\end{mydef}
}

\newenvironment{Korollar}[1]{%
		\begin{cor}[#1]
}{%
		\end{cor}
}



\newshadedtheorem{cor}[sat]{Korollar}

\theoremstyle{break}
\theoremsymbol{\ensuremath{\blacksquare}}
\newtheorem*{bevis}{Proof}
\theoremsymbol{\ensuremath{\square}}

\newtheorem{eks}[sat]{Eksempel}
\newenvironment{Eksempel}{%
		\begin{eks}
}{%
		\end{eks}
}

\newtheorem{bem}[sat]{Remark}
\newenvironment{Bemarkning}{%
		\begin{bem}
}{%
		\end{bem}
}

\renewcommand{\qedsymbol}{}

\setlength{\delimitershortfall}{0pt} %SÃ¸rger for at matrix med partial diff lukker helt til i toppen

%smÃ¥ bogstaver med fed
\newcommand{\ba}{\mathbf{a}}
\newcommand{\bb}{\mathbf{b}}
\newcommand{\bc}{\mathbf{c}}
\newcommand{\bd}{\mathbf{d}}
\newcommand{\bee}{\mathbf{e}}
\newcommand{\bff}{\mathbf{f}}
\newcommand{\bg}{\mathbf{g}}
\newcommand{\bh}{\mathbf{h}}
\newcommand{\bi}{\mathbf{i}}
\newcommand{\bj}{\mathbf{j}}
\newcommand{\bk}{\mathbf{k}}
\newcommand{\bl}{\mathbf{l}}
\newcommand{\bm}{\mathbf{m}}
\newcommand{\bn}{\mathbf{n}}
\newcommand{\bo}{\mathbf{o}}
\newcommand{\bp}{\mathbf{p}}
\newcommand{\bq}{\mathbf{q}}
\newcommand{\br}{\mathbf{r}}
\newcommand{\bs}{\mathbf{s}}
\newcommand{\bttt}{\mathbf{t}}
\newcommand{\bu}{\mathbf{u}}
\newcommand{\bv}{\mathbf{v}}
\newcommand{\bw}{\mathbf{w}}
\newcommand{\bx}{\mathbf{x}}
\newcommand{\by}{\mathbf{y}}
\newcommand{\bz}{\mathbf{z}}
%store bogstaver med fed
\newcommand{\bA}{\mathbf{A}}
\newcommand{\bB}{\mathbf{B}}
\newcommand{\bC}{\mathbf{C}}
\newcommand{\bD}{\mathbf{D}}
\newcommand{\bE}{\mathbf{E}}
\newcommand{\bF}{\mathbf{F}}
\newcommand{\bG}{\mathbf{G}}
\newcommand{\bH}{\mathbf{H}}
\newcommand{\bI}{\mathbf{I}}
\newcommand{\bJ}{\mathbf{J}}
\newcommand{\bK}{\mathbf{K}}
\newcommand{\bL}{\mathbf{L}}
\newcommand{\bM}{\mathbf{M}}
\newcommand{\bN}{\mathbf{N}}
\newcommand{\bO}{\mathbf{O}}
\newcommand{\bP}{\mathbf{P}}
\newcommand{\bQ}{\mathbf{Q}}
\newcommand{\bR}{\mathbf{R}}
\newcommand{\bS}{\mathbf{S}}
\newcommand{\bTT}{\mathbf{T}}
\newcommand{\bU}{\mathbf{U}}
\newcommand{\bV}{\mathbf{V}}
\newcommand{\bW}{\mathbf{W}}
\newcommand{\bX}{\mathbf{X}}
\newcommand{\bY}{\mathbf{Y}}
\newcommand{\bZ}{\mathbf{Z}}

%SmÃ¥ bogstaver med tilde og fed
\newcommand{\tba}{\widetilde{\mathbf{a}}}
\newcommand{\tbb}{\widetilde{\mathbf{b}}}
\newcommand{\tbc}{\widetilde{\mathbf{c}}}
\newcommand{\tbd}{\widetilde{\mathbf{d}}}
\newcommand{\tbe}{\widetilde{\mathbf{e}}}
\newcommand{\tbf}{\widetilde{\mathbf{f}}}
\newcommand{\tbg}{\widetilde{\mathbf{g}}}
\newcommand{\tbh}{\widetilde{\mathbf{h}}}
\newcommand{\tbi}{\widetilde{\mathbf{i}}}
\newcommand{\tbj}{\widetilde{\mathbf{j}}}
\newcommand{\tbk}{\widetilde{\mathbf{k}}}
\newcommand{\tbl}{\widetilde{\mathbf{l}}}
\newcommand{\tbm}{\widetilde{\mathbf{m}}}
\newcommand{\tbn}{\widetilde{\mathbf{n}}}
\newcommand{\tbo}{\widetilde{\mathbf{o}}}
\newcommand{\tbp}{\widetilde{\mathbf{p}}}
\newcommand{\tbq}{\widetilde{\mathbf{q}}}
\newcommand{\tbr}{\widetilde{\mathbf{r}}}
\newcommand{\tbs}{\widetilde{\mathbf{s}}}
\newcommand{\tbt}{\widetilde{\mathbf{t}}}
\newcommand{\tbu}{\widetilde{\mathbf{u}}}
\newcommand{\tbv}{\widetilde{\mathbf{v}}}
\newcommand{\tbw}{\widetilde{\mathbf{w}}}
\newcommand{\tbx}{\widetilde{\mathbf{x}}}
\newcommand{\tby}{\widetilde{\mathbf{y}}}
\newcommand{\tbz}{\widetilde{\mathbf{z}}}

%SmÃ¥ bogstaver med hat
\newcommand{\ha}{\widehat{a}}
\newcommand{\hb}{\widehat{b}}
\newcommand{\hc}{\widehat{c}}
\newcommand{\hd}{\widehat{d}}
\newcommand{\he}{\widehat{e}}
\newcommand{\hf}{\widehat{f}}
\newcommand{\hg}{\widehat{g}}
\newcommand{\hh}{\widehat{h}}
\newcommand{\hi}{\widehat{i}}
\newcommand{\hj}{\widehat{j}}
\newcommand{\hk}{\widehat{k}}
\newcommand{\hl}{\widehat{l}}
\newcommand{\hm}{\widehat{m}}
\newcommand{\hn}{\widehat{n}}
\newcommand{\ho}{\widehat{o}}
\newcommand{\hp}{\widehat{p}}
\newcommand{\hq}{\widehat{q}}
\newcommand{\hr}{\widehat{r}}
\newcommand{\hs}{\widehat{s}}
\newcommand{\htt}{\widehat{t}}
\newcommand{\hu}{\widehat{u}}
\newcommand{\hv}{\widehat{v}}
\newcommand{\hw}{\widehat{w}}
\newcommand{\hx}{\widehat{x}}
\newcommand{\hy}{\widehat{y}}
\newcommand{\hz}{\widehat{z}}

%SmÃ¥ bogstaver med tilde
\newcommand{\ta}{\widetilde{a}}
\newcommand{\tb}{\widetilde{b}}
\newcommand{\tc}{\widetilde{c}}
\newcommand{\td}{\widetilde{d}}
\newcommand{\te}{\widetilde{e}}
\newcommand{\tf}{\widetilde{f}}
\newcommand{\tg}{\widetilde{g}}
\newcommand{\thh}{\widetilde{h}}
\newcommand{\ti}{\widetilde{i}}
\newcommand{\tj}{\widetilde{j}}
\newcommand{\tk}{\widetilde{k}}
\newcommand{\tl}{\widetilde{l}}
\newcommand{\tm}{\widetilde{m}}
\newcommand{\tn}{\widetilde{n}}
\newcommand{\tooo}{\widetilde{o}}
\newcommand{\tp}{\widetilde{p}}
\newcommand{\tq}{\widetilde{q}}
\newcommand{\trr}{\widetilde{r}}
\newcommand{\ts}{\widetilde{s}}
\newcommand{\ttt}{\widetilde{t}}
\newcommand{\tu}{\widetilde{u}}
\newcommand{\tv}{\widetilde{v}}
\newcommand{\tw}{\widetilde{w}}
\newcommand{\tx}{\widetilde{x}}
\newcommand{\ty}{\widetilde{y}}
\newcommand{\tz}{\widetilde{z}}

%SmÃ¥ bogstaver med fed og overline
\newcommand{\obs}{\overline{\mathbf{s}}}

%Store bogstaver med tilde og fed
\newcommand{\tbA}{\widetilde{\mathbf{A}}}
\newcommand{\tbB}{\widetilde{\mathbf{B}}}
\newcommand{\tbC}{\widetilde{\mathbf{C}}}
\newcommand{\tbD}{\widetilde{\mathbf{D}}}
\newcommand{\tbE}{\widetilde{\mathbf{E}}}
\newcommand{\tbF}{\widetilde{\mathbf{F}}}
\newcommand{\tbG}{\widetilde{\mathbf{G}}}
\newcommand{\tbH}{\widetilde{\mathbf{H}}}
\newcommand{\tbI}{\widetilde{\mathbf{I}}}
\newcommand{\tbJ}{\widetilde{\mathbf{J}}}
\newcommand{\tbK}{\widetilde{\mathbf{K}}}
\newcommand{\tbL}{\widetilde{\mathbf{L}}}
\newcommand{\tbM}{\widetilde{\mathbf{M}}}
\newcommand{\tbN}{\widetilde{\mathbf{N}}}
\newcommand{\tbO}{\widetilde{\mathbf{O}}}
\newcommand{\tbP}{\widetilde{\mathbf{P}}}
\newcommand{\tbQ}{\widetilde{\mathbf{Q}}}
\newcommand{\tbR}{\widetilde{\mathbf{R}}}
\newcommand{\tbS}{\widetilde{\mathbf{S}}}
\newcommand{\tbT}{\widetilde{\mathbf{T}}}
\newcommand{\tbU}{\widetilde{\mathbf{U}}}
\newcommand{\tbV}{\widetilde{\mathbf{V}}}
\newcommand{\tbW}{\widetilde{\mathbf{W}}}
\newcommand{\tbX}{\widetilde{\mathbf{X}}}
\newcommand{\tbY}{\widetilde{\mathbf{Y}}}
\newcommand{\btZ}{\widetilde{\mathbf{Z}}}
\newcommand{\tbZ}{\widetilde{\mathbf{Z}}}


%Fede tal
\newcommand{\bnul}{\mathbf{0}}
\newcommand{\bet}{\mathbf{1}}
\newcommand{\bto}{\mathbf{2}}
\newcommand{\btre}{\mathbf{3}}
\newcommand{\bfire}{\mathbf{4}}
\newcommand{\bfem}{\mathbf{5}}
\newcommand{\bseks}{\mathbf{6}}
\newcommand{\bsyv}{\mathbf{7}}
\newcommand{\botte}{\mathbf{8}}
\newcommand{\bni}{\mathbf{9}}
%black board bold bogstaver
\newcommand{\A}{\mathbb{A}}
\newcommand{\B}{\mathbb{B}}
\newcommand{\C}{\mathbb{C}}
\newcommand{\bbE}{\mathbb{E}}
\newcommand{\bbG}{\mathbb{G}}
\newcommand{\bbH}{\mathbb{H}}
\newcommand{\Rn}{\mathbb{R}^n}
\newcommand{\R}{\mathbb{R}}
\newcommand{\Z}{\mathbb{Z}}
\newcommand{\N}{\mathbb{N}}
\newcommand{\Q}{\mathbb{Q}}

%Mathcal bogstaver
\newcommand{\cA}{\mathcal{A}}
\newcommand{\cB}{\mathcal{B}}
\newcommand{\cC}{\mathcal{C}}
\newcommand{\cD}{\mathcal{D}}
\newcommand{\cE}{\mathcal{E}}
\newcommand{\cF}{\mathcal{F}}
\newcommand{\cG}{\mathcal{G}}
\newcommand{\cH}{\mathcal{H}}
\newcommand{\cI}{\mathcal{I}}
\newcommand{\cJ}{\mathcal{J}}
\newcommand{\cK}{\mathcal{K}}
\newcommand{\cL}{\mathcal{L}}
\newcommand{\cM}{\mathcal{M}}
\newcommand{\cN}{\mathcal{N}}
\newcommand{\cO}{\mathcal{O}}
\newcommand{\cP}{\mathcal{P}}
\newcommand{\cQ}{\mathcal{Q}}
\newcommand{\cR}{\mathcal{R}}
\newcommand{\cS}{\mathcal{S}}
\newcommand{\cT}{\mathcal{T}}
\newcommand{\cU}{\mathcal{U}}
\newcommand{\cV}{\mathcal{V}}
\newcommand{\cW}{\mathcal{W}}
\newcommand{\cX}{\mathcal{X}}
\newcommand{\cY}{\mathcal{Y}}
\newcommand{\cZ}{\mathcal{Z}}

%Hat bogstaver
\newcommand{\hcK}{\widehat{\cK}}
\newcommand{\hK}{\widehat{K}}
\newcommand{\hL}{\widehat{L}}
\newcommand{\hF}{\widehat{F}}
\newcommand{\hG}{\widehat{G}}
\newcommand{\hJ}{\widehat{J}}

%Mathscr
\newcommand{\sA}{\mathscr{A}}
\newcommand{\sB}{\mathscr{B}}
\newcommand{\sC}{\mathscr{C}}
\newcommand{\sD}{\mathscr{D}}
\newcommand{\sE}{\mathscr{E}}
\newcommand{\sF}{\mathscr{F}}
\newcommand{\sG}{\mathscr{G}}
\newcommand{\sH}{\mathscr{H}}
\newcommand{\sI}{\mathscr{I}}
\newcommand{\sJ}{\mathscr{J}}
\newcommand{\sK}{\mathscr{K}}
\newcommand{\sL}{\mathscr{L}}
\newcommand{\sM}{\mathscr{M}}
\newcommand{\sN}{\mathscr{N}}
\newcommand{\sO}{\mathscr{O}}
\newcommand{\sP}{\mathscr{P}}
\newcommand{\sQ}{\mathscr{Q}}
\newcommand{\sR}{\mathscr{R}}
\newcommand{\sS}{\mathscr{S}}
\newcommand{\sT}{\mathscr{T}}
\newcommand{\sU}{\mathscr{U}}
\newcommand{\sV}{\mathscr{V}}
\newcommand{\sW}{\mathscr{W}}
\newcommand{\sX}{\mathscr{X}}
\newcommand{\sY}{\mathscr{Y}}
\newcommand{\sZ}{\mathscr{Z}}


%Store grÃ¦ske bogstaver
\newcommand{\bT}{\Theta}

%GrÃ¦ske bogstaver med fed
\newcommand{\bmu}{\boldsymbol{\mu}}
\newcommand{\btheta}{\boldsymbol{\theta}}
\newcommand{\bgamma}{\boldsymbol{\gamma}}
\newcommand{\bphi}{\boldsymbol{\varphi}}
\newcommand{\bbeta}{\boldsymbol{\beta}}
\newcommand{\be}{\boldsymbol{\varepsilon}}
\newcommand{\bepsilon}{\boldsymbol{\varepsilon}}

%SmÃ¥ grÃ¦ske bogstaver med hat
\newcommand{\gh}{\widehat{\gamma}}
\newcommand{\sh}{\widehat{\sigma}}
\newcommand{\rh}{\widehat{\rho}}
\newcommand{\hgamma}{\widehat{\gamma}}
\newcommand{\hsigma}{\widehat{\sigma}}
\newcommand{\hrho}{\widehat{\rho}}
\newcommand{\hbeta}{\widehat{\beta}}
\newcommand{\hepsilon}{\widehat{\varepsilon}}
\newcommand{\halpha}{\widehat{\alpha}}


%Store grÃ¦ske bogstaver med hat
\newcommand{\Gh}{\widehat{\Gamma}}
\newcommand{\Rh}{\widehat{R}}
\newcommand{\hGamma}{\widehat{\Gamma}}
\newcommand{\hRho}{\widehat{R}}

%Store grÃ¦ske bogstaver med tilde
\newcommand{\tAlpha}{\widetilde{A}}
\newcommand{\tBeta}{\widetilde{B}}
\newcommand{\tGamma}{\widetilde{\Gamma}}
\newcommand{\tDelta}{\widetilde{\Delta}}
\newcommand{\tEpsilon}{\widetilde{\E}}
\newcommand{\tOmega}{\widetilde{\Omega}}

%GrÃ¦ske bogstaver med tilde og fed
\newcommand{\tbmu}{\widetilde{\boldsymbol{\mu}}}
\newcommand{\btt}{\boldsymbol{\widetilde{\theta}}}


%GrÃ¦ske bogstaver med fed og overline
\newcommand{\obphi}{\overline{\boldsymbol{\phi}}}


%Store grÃ¦ske bogstaver med tilde og fed

%GrÃ¦ske bogstaver med hat og fed
\newcommand{\bth}{\boldsymbol{\widehat{\theta}}}
\newcommand{\hbtheta}{\widehat{\boldsymbol{\theta}}}
\newcommand{\bbh}{\widehat{\boldsymbol{\beta}}}
\newcommand{\hbbeta}{\widehat{\boldsymbol{\beta}}}
\newcommand{\bsh}{\widehat{\boldsymbol{\sigma}}}
\newcommand{\hbsigma}{\widehat{\boldsymbol{\sigma}}}
\newcommand{\brh}{\widehat{\boldsymbol{\rho}}}
\newcommand{\hbrho}{\widehat{\boldsymbol{\rho}}}
\newcommand{\bgh}{\widehat{\boldsymbol{\gamma}}}
\newcommand{\hbgamma}{\widehat{\boldsymbol{\gamma}}}
\newcommand{\bmh}{\widehat{\boldsymbol{\mu}}}
\newcommand{\hbmu}{\widehat{\boldsymbol{\mu}}}
\newcommand{\bphih}{\widehat{\boldsymbol{\varphi}}}
\newcommand{\hbphi}{\widehat{\boldsymbol{\varphi}}}

%Store grÃ¦ske bogstaver med hat og fed

%GrÃ¦ske bogstaver med hat og tilde
\newcommand{\sht}{\widetilde{\widehat{\sigma}}}
%Ting der skal redefineres
\renewcommand{\epsilon}{\varepsilon}
\renewcommand{\phi}{\varphi}
\renewcommand{\Re}{\textup{Re}}

%Textup kommandoer
\newcommand{\E}{\textup{E}}
\newcommand{\Var}{\textup{Var}}
\newcommand{\Cov}{\textup{Cov}}
\newcommand{\bspan}{\textup{span}}
\newcommand{\rank}{\textup{rank}}
\newcommand{\range}{\textup{range}}
\newcommand{\AIC}{\textup{AIC}}


%Ting i declareMathOperator
\DeclareMathOperator*{\slim}{s-lim}
\DeclareMathOperator*{\flim}{f-lim}
\DeclareMathOperator*{\inte}{int}
\DeclareMathOperator*{\epi}{epi}
\DeclareMathOperator*{\GL}{GL_n(\mathbb{R})}
\DeclareMathOperator*{\SL}{SL_n(\mathbb{R})}\DeclareMathOperator*{\On}{O_n(\mathbb{R})}\DeclareMathOperator*{\SON
}{SO_n(\mathbb{R})}
\DeclareMathOperator*{\Ker}{Ker}
\DeclareMathOperator*{\so}{SO_2(\mathbb{R})}
\DeclareMathOperator*{\oo}{O_2(\mathbb{R})}
\DeclareMathOperator*{\Isom}{Isom(\mathbb{R}^2)}
\DeclareMathOperator*{\Sym}{Sym}
\DeclareMathOperator*{\tr}{tr}
\DeclareMathOperator*{\gl}{GL_2(\mathbb{Z})}

\DeclareMathOperator*{\Col}{Col}
%\DeclareMathOperator*{\Var}{Var}
\DeclareMathOperator*{\Int}{Int}
%\DeclareMathOperator*{\Cov}{Cov}
\DeclareMathOperator*{\Corr}{Corr}




\newcommand{\id}{\mathrm{id}}

\newcommand{\tal}{\setcounter{section}{1}
\setcounter{sat}{0}}


\newcommand{\bbt}{\bar{\boldsymbol{\theta}}}

\newcommand{\bhx}{\widehat{\mathbf{x}}}
\newcommand{\btx}{\widetilde{\mathbf{x}}}


\newcommand{\pdif}[1]{\frac{\partial}{\partial#1} }

\newcommand{\abs}[1]{\vert #1 \vert}
\newcommand{\nor}[1]{\Vert #1 \Vert}
\newcommand{\lr}[1]{\langle #1 \rangle}
