# Supplementary material for: Second order semi-parametric inference for multivariate log Gaussian Cox processes
Source: arXiv:2012.02155 source file (2022-01-03)
Supplement: Supplementary file 6 [file preamble.tex]

% !TEX TS-program = pdflatexmk
%  A simple AAU report template.
%  2015-05-08 v. 1.2.0
%  Copyright 2010-2015 by Jesper Kjær Nielsen <jkn@es.aau.dk>
%
%  This is free software: you can redistribute it and/or modify
%  it under the terms of the GNU General Public License as published by
%  the Free Software Foundation, either version 3 of the License, or
%  (at your option) any later version.
%
%  This is distributed in the hope that it will be useful,
%  but WITHOUT ANY WARRANTY; without even the implied warranty of
%  MERCHANTABILITY or FITNESS FOR A PARTICULAR PURPOSE.  See the
%  GNU General Public License for more details.
%
%  You can find the GNU General Public License at <http://www.gnu.org/licenses/>.
%
\documentclass[11pt,twoside,a4paper,openright]{article}
%%%%%%%%%%%%%%%%%%%%%%%%%%%%%%%%%%%%%%%%%%%%%%%%
% Language, Encoding and Fonts
% http://en.wikibooks.org/wiki/LaTeX/Internationalization
%%%%%%%%%%%%%%%%%%%%%%%%%%%%%%%%%%%%%%%%%%%%%%%%
% Select encoding of your inputs. Depends on
% your operating system and its default input
% encoding. Typically, you should use
%   Linux  : utf8 (most modern Linux distributions)
%            latin1 
%   Windows: ansinew
%            latin1 (works in most cases)
%   Mac    : applemac
% Notice that you can manually change the input
% encoding of your files by selecting "save as"
% an select the desired input encoding. 
\usepackage[latin1]{inputenc}
%\usepackage[utf8]{inputenc}
%\usepackage[applemac]{inputenc} 
% Make latex understand and use the typographic
% rules of the language used in the document.
\usepackage[english]{babel}
% Use the palatino font
%\usepackage[sc]{mathpazo}
%\linespread{1.05}         % Palatino needs more leading (space between lines)
% Choose the font encoding
\usepackage[T1]{fontenc}
\usepackage{ae,aecompl}   %Flere fonts 
\usepackage{ragged2e,anyfontsize}			% Justering af elementer
\usepackage{fixltx2e}						% Retter forskellige fejl i LaTeX-kernen
\usepackage{lmodern}
\usepackage{graphicx,wrapfig,lipsum}
\usepackage{subcaption}
%%%%%%%%%%%%%%%%%%%%%%%%%%%%%%%%%%%%%%%%%%%%%%%%
% Graphics and Tables
% http://en.wikibooks.org/wiki/LaTeX/Importing_Graphics
% http://en.wikibooks.org/wiki/LaTeX/Tables
% http://en.wikibooks.org/wiki/LaTeX/Colors
%%%%%%%%%%%%%%%%%%%%%%%%%%%%%%%%%%%%%%%%%%%%%%%%
% load a colour package
\usepackage[dvipsnames]{xcolor}
\definecolor{aaublue}{RGB}{33,26,82}% dark blue
% The standard graphics inclusion package
\usepackage{graphicx}
% Set up how figure and table captions are displayed
\usepackage{caption}
\captionsetup{%
  font=footnotesize,% set font size to footnotesize
  labelfont=bf % bold label (e.g., Figure 3.2) font
}
% Make the standard latex tables look so much better
\usepackage{array,booktabs}
% Enable the use of frames around, e.g., theorems
% The framed package is used in the example environment
\usepackage{framed}

%%%%%%%%%%%%%%%%%%%%%%%%%%%%%%%%%%%%%%%%%%%%%%%%
% Mathematics
% http://en.wikibooks.org/wiki/LaTeX/Mathematics
%%%%%%%%%%%%%%%%%%%%%%%%%%%%%%%%%%%%%%%%%%%%%%%%
% Defines new environments such as equation,
% align and split 
\usepackage{amsmath}
% Adds new math symbols
\usepackage{amssymb}
\usepackage{mathtools}
\usepackage{ mathrsfs }


% Use theorems in your document
% The ntheorem package is also used for the example environment
% When using thmmarks, amsmath must be an option as well. Otherwise \eqref doesn't work anymore.
\usepackage[framed,amsmath,thmmarks]{ntheorem}


%%%%%%%%%%%%%%%%%%%%%%%%%%%%%%%%%%%%%%%%%%%%%%%%
% Page Layout
% http://en.wikibooks.org/wiki/LaTeX/Page_Layout
%%%%%%%%%%%%%%%%%%%%%%%%%%%%%%%%%%%%%%%%%%%%%%%%
% Change margins, papersize, etc of the document
\usepackage[
	top=30mm,
	bottom=30mm,  
  inner=25mm,% left margin on an odd page
  outer=35mm,% right margin on an odd page
  ]{geometry}
% Modify how \chapter, \section, etc. look
% The titlesec package is very configureable
\usepackage{titlesec}
\titleformat{\chapter}[display]{\normalfont\huge\bfseries}{\chaptertitlename\ \thechapter}{20pt}{\Huge}
\titleformat*{\section}{\normalfont\Large\bfseries}
\titleformat*{\subsection}{\normalfont\large\bfseries}
\titleformat*{\subsubsection}{\normalfont\normalsize\bfseries}
%\titleformat*{\paragraph}{\normalfont\normalsize\bfseries}
%\titleformat*{\subparagraph}{\normalfont\normalsize\bfseries}
%Modify the spacing above chapter
\titlespacing*{\chapter}{0pt}{-50pt}{20pt}
\addto\captionsdanish{%
\renewcommand\chaptername{}}
%Removing "Chapter X" on every chapter numbered page and adding the chapternumber to the left of title
\titleformat{\chapter}[display]{\normalfont\huge\bfseries}{ }{20pt}{ \thechapter.\ \Huge}
%Same as above but for numberless chapters. No number is addet to the left of the title.
\titleformat{name=\chapter,numberless}[display]{\normalfont\huge\bfseries}{ }{20pt}{\Huge}


% Clear empty pages between chapters
\let\origdoublepage\cleardoublepage
\newcommand{\clearemptydoublepage}{%
  \clearpage
  {\pagestyle{empty}\origdoublepage}%
}
\let\cleardoublepage\clearemptydoublepage

% Change the headers and footers
\usepackage{fancyhdr}
\pagestyle{fancy}
\fancyhf{} %delete everything
\renewcommand{\headrulewidth}{0pt} %remove the horizontal line in the header
\fancyhead[RE]{\small\nouppercase\leftmark} %even page - chapter title
\fancyhead[LO]{\small\nouppercase\rightmark} %uneven page - section title
\fancyhead[LE,RO]{\thepage} %page number on all pages
% Do not stretch the content of a page. Instead,
% insert white space at the bottom of the page
\raggedbottom
% Enable arithmetics with length. Useful when
% typesetting the layout.
\usepackage{calc}

%%%%%%%%%%%%%%%%%%%%%%%%%%%%%%%%%%%%%%%%%%%%%%%%
% Bibliography
% http://en.wikibooks.org/wiki/LaTeX/Bibliography_Management
%%%%%%%%%%%%%%%%%%%%%%%%%%%%%%%%%%%%%%%%%%%%%%%%
%\usepackage[backend=bibtex,
%  bibencoding=utf8,
%citestyle=authoryear
%  ]{biblatex}
%\addbibresource{bib/mybib}

\usepackage[square]{natbib}
%\usepackage[apalike]{dk-bib}
% Appearance of the bibliography
%\bibliographystyle{dlfltxbbibtex}
%\bibliographystyle{dk-apali}
%\bibliographystyle{plain}
%\bibliographystyle{unsrtnat}
\bibliographystyle{apa}
%%%%%%%%%%%%%%%%%%%%%%%%%%%%%%%%%%%%%%%%%%%%%%%%
% Misc
%%%%%%%%%%%%%%%%%%%%%%%%%%%%%%%%%%%%%%%%%%%%%%%%
% Add bibliography and index to the table of
% contents
\usepackage[nottoc]{tocbibind}
% Add the command \pageref{LastPage} which refers to the
% page number of the last page
\usepackage{lastpage}
% Add todo notes in the margin of the document
\usepackage[
%  disable, %turn off todonotes
  colorinlistoftodos, %enable a coloured square in the list of todos
  textwidth=\marginparwidth, %set the width of the todonotes
  textsize=scriptsize, %size of the text in the todonotes
  ]{todonotes}

%%%%%%%%%%%%%%%%%%%%%%%%%%%%%%%%%%%%%%%%%%%%%%%%
% Hyperlinks
% http://en.wikibooks.org/wiki/LaTeX/Hyperlinks
%%%%%%%%%%%%%%%%%%%%%%%%%%%%%%%%%%%%%%%%%%%%%%%%
% Enable hyperlinks and insert info into the pdf
% file. Hypperref should be loaded as one of the 
% last packages
\usepackage{hyperref}
\hypersetup{%
	%pdfpagelabels=true,%
	plainpages=false,%
	pdfauthor={Author(s)},%
	pdftitle={Title},%
	pdfsubject={Subject},%
	bookmarksnumbered=true,%
	colorlinks=false,%
	citecolor=black,%
	filecolor=black,%
	linkcolor=black,% you should probably change this to black before printing
	urlcolor=black,%
	pdfstartview=FitH%
}
%%Lister
\usepackage{enumitem}

%%Tegnepakke
\usepackage{tikz}
\usepackage{tkz-berge}
\usetikzlibrary{shapes.geometric, intersections}
%\usepackage{xspace}
%\newcommand{\A}{\ensuremath{\mathcal{A}}\xspace}
%\newcommand{\B}{\ensuremath{\mathcal{B}}\xspace}
%\newcommand\pa[1]{\ensuremath{\left(#1\right)}}
\usepackage[font = scriptsize]{subcaption}
\usepackage{tkz-tab}
\usepackage{pgfplots}
%\usepgfplotslibrary{fillbetween}
\pgfplotsset{
	width=7cm,
	compat=1.3,
	inner axis line style={=>},
	axis lines=middle,
	scale only axis,
 	xlabel={\small $x$},
  	ylabel={\small $y$},
	every axis/.append style={font=\tiny},
}
\usetikzlibrary{decorations.markings}
\makeatletter
\tikzset{
    nomorepostaction/.code={\let\tikz@postactions\pgfutil@empty},
    plotlabel/.style 2 args={
        every path/.append style={
            postaction={
                nomorepostaction,
                decorate,
                decoration={
                    markings,
                    mark=at position #1 with {
                        \pgftransformresetnontranslations
           \pgfsetlinewidth{0.4pt}
           \pgfsetstrokecolor{black}
           \pgfpathmoveto{\pgfpointorigin}
           \pgfpathlineto{\pgfpoint{-0.3cm}{0.6cm}}
           \pgfusepath{stroke}
           \pgftransformshift{\pgfpoint{-0.3cm}{0.6cm}}
                        \pgfnode{rectangle}{east}{#2}{}{}
                    }
                }
            }
        }
    }
}
\makeatother
\usetikzlibrary{calc}
\usepackage{float}
\usetikzlibrary{external}
% Enable the library
\tikzexternalize

%fjerner warnings fra fancyhdr
\setlength{\headheight}{15pt}
\usepackage{multirow}
\usepackage{mathdots}
\usepackage{subcaption}
\usepackage{mathrsfs}
%%Listings
\usepackage{listings}
\lstset{% general command to set parameter(s)
basicstyle=\ttfamily, % print whole listing small
keywordstyle=\color{blue},
% underlined bold black keywords
identifierstyle=, % nothing happens
commentstyle=\color{ForestGreen}, % white comments
stringstyle=\ttfamily, % typewriter type for strings
showstringspaces=false,
emph={in},
emphstyle=\color{blue},
numbers=left,
 numberstyle=\small, 
numbersep=5pt,
frame=lt,
breaklines=true
} % no special string spaces

%\usepackage{slashbox}
\usepackage{rotating}
\usepackage{pdflscape}
\usepackage{geometry}
\usepackage{hhline}

%\overfullrule=5pt
